# Supplementary material for: On Optimizing the Communication of Model Parallelism
Source: arXiv:2211.05322 source file (2024-08-18)
Supplement: Supplementary file 1 [file appendix.notations.tex]

\section{Notation table}
\begin{table*}[h!]
\begin{tabular}{|p{8.5cm}|p{8.5cm}|}
\hline
Notation                                   & Description                                                                      \\ \hline
$mesh_A$ and $mesh_B$                      & device meshes                                                                    \\ \hline
$T_{broadcast}(m)$, $T_{sendrecv}(m)$, $T_{sendrecv+local allgather}(m)$, $T_{sendrecv+global allgather}(m)$ &
  time for these methods to finish a "1-to-m" data send task \\ \hline
T                                          & time for one data to be sent from one host to another one via infiniband         \\ \hline
$N_i$ in $i_{th}$ "N-to-M data send task", & The number of devices that could potentially be the sender.                      \\ \hline
$M_i$ in $i_{th}$ "N-to-M data send task"  & The number of devices that ask for the data.                                     \\ \hline
$D_{0,1,2,..M}$ &
  ring-based nccl operation will chain all devices together, this is the order for these devices on the chain. $D_0$ is the sender and $D_{1,2,\dots, M}$ are receivers. During the data transfer, $D_i$ receives data from $D_{i-1}$ and sends data to $D_{i+1}$ \\ \hline
$K$                                        & the whole data A is splitted into $K$ pieces during nccl broadcast               \\ \hline
$sd_{ix}\in A, x\in \{0,1,\dots, n_i-1\}$ & the $x_{th}$ nic behind which devices contains data copy for the $i_{th}$ task   \\ \hline
$td_{i,y}\in B, y\in \{0,1,\dots, m_i-1\}$ & the $y_{th}$ nic behind which devices ask for the data copy in the $i_{th}$ task \\ \hline
$T_i$                                      & task $i$ takes $T_i$ time to finish                                              \\ \hline
$S_i$ &
  start task $i$ at $S_i$; And task $i$ takes up $[S_i, S_i+T_i]$ on the timelines of $sd_{i, x_i}$ and all $td_{i, y}, y\in \{0,1,\dots, m_i-1\}$ \\ \hline
$I_j$                                      & the tasks that are assigned to $j_{th}$ NIC is $I_j$                             \\ \hline
\end{tabular}
\end{table*}
